# Supplementary material for: Fundamental Limits in Formal Verification of Message-Passing Neural Networks
Source: arXiv:2206.05070 source file (2022-10-04)
Supplement: Supplementary file 1 [file supplementary.tex]

\begin{lemma}
	Let $r \in \mathbb{R}$ and $(r_1, \dotsc, r_k) \in \mathbb{R}^k$ for some $k$.
	%$\gad{r \in M} = 0$ if and only if $r \in M$, 
	$\gad{(r_1, \dotsc, r_k)} = 0$ if and only if 
	exactly one $r_i = 1$ and all other are $0$,
	$\gad{r = m} = 0$ if and only if $r=m$, 
	$\gad{r \leq m} = 0$ if and only if $r \leq m$ and
	if $g(r) \geq 1$ or if $g(r)=0$ and all $f_i(r_i)=0$ then it holds that
	$\gad{g(r) \rightarrow f_1(r_1) + \dotsb + f_k(r_k)} = 0$.
	Furthermore, $\gad{x = m}, \gad{x \leq m}$, %$\gad{x \in M}$ 
	are positive and bounded and gadget
	$\gad{g(x) \rightarrow f_1(x_1) + \dotsb + f_k(x_k)}$ is positive.
	If $|m-r| \geq 1$ then $\gad{r = m} \geq 1$. %and if $\min_M(|r-i_j|) \geq 1$ then $\gad{r \in M} \geq 1$.  
	\label{sec:undecidable;lem:gadget_prop}
\end{lemma}
\begin{proof}
	Let $\mathcal{C} = (C_1, \dotsc, C_m, \{\varphi_{ic} \mid i \in {1, \dotsc, m}, c \in C_i\}, n, \chi)$ like above. 
	The GNN $N_\mathcal{C}$ has input dimension $|C_1| + \dotsb
	+ |C_m| + n$ and $\hat{i} = \max\{\bigcup_{w \in }\}$ layers followed by the readout layer.
	We describe the GNN $N_\mathcal{C}$ by specifying the outputs of each layer $l_i$ and the single output $y^r$ of the readout layer.
	For all such outputs holds that they are given by a sum of gadgets as defined above. As all used gadgets are positive, this implies that an output can only be 0
	if all gadgets output 0 or, according to Lemma~\ref{sec:undecidable;lem:gadget_prop}, their respective property is satisfied.
	If not stated otherwise, an output dimension $y^i$ of some layer $l_i$ implies that there are output dimensions $y^j = y^{j-1}$ for layers $j > i$. 
	In other words, the dimension $y^i$ is transported through the following layers without further adjustments.
	
	Layer $l_1$ includes an output dimension $y^1_\text{color}$ computed by $\sum_{i \in \{1, \dotsc, m\}} \gad{\boldsymbol{x}_{C_i}}$. The output
	$y^r$ includes a gadget $\smallgad{y^{\hat{i}}_\text{color}=0}$. This ensures that if $N_\mathcal{C}(G)=0$ that each node of $G$ can be colored 
	with exactly one color of each $C_i$, namely the one corresponding to the dimension of $\boldsymbol{x}_{C_i}$ that is equal to $1$. 
	Next, we argue how $N_\mathcal{C}$ represents a node condition $\varphi_{ic} = \psi^1_1 \land \dotsb \land \psi^k_1 \land \psi^1_2 \land \dotsb \land \psi^l_2$.
	The last layer includes an output dimension $y^{\hat{i}}_{ic} = \gad{\gad{x_{ic}=1} \rightarrow f^1_1(x^1_1) + \dotsb + f^l_2(x^l_2)}$
	where the $f$ gadgets are defined by the subformulas $\psi^j_1$ and $\psi^j_2$.
	If $\psi^j_1 = c$ for some color $c$ then $x^j_1$ is the input dimension corresponding
	to color $c$ and $f^j_1(x^j_1) = \smallgad{x^j_1=1}$ and if $\psi^j_1 = \neg c$ then $f^j_1(x^j_1) = \smallgad{x^j_1=0}$. Next, consider the case $\psi^j_1 = (w,p)$.
	If $|w|=1$ and $w=c$ then $x^j_1$ is the neighbourhood dimension corresponding to color $c$ and $f^j_1(x^j_1) = \smallgad{x^j_1 = p}$. If
	$w=w_1 \dotsb w_q$ with $q \geq 2$ then $f^j_1(x^j_1)=\smallgad{{y'}^{\hat{i}}_{ic,j1} = p}$ where ${y'}^{\hat{i}}_{ic,j1}$ is given as follows: 
	In layer $l_1$ we have an output $y^1_{ic,j1} = \relu(\relu(x_{w_q}) - \relu(x_{w_q}-(p+1)))$ and in layer $2 \leq i \leq q$ we have the output 
	$y^i_{ic,j1} = \relu(\relu({y'}^i_{ic,j1}) - \relu({y'}^i_{ic,j1}-(p+1)) - (p+1)\relu(1-x_{w_{q-(i-1)}}))$. It can be seen that output $y^i_{ic,j1}$ is 
	equal to the number (bounded by $p+1$) of paths of the form $w_{q-(i-1)} \dotsb w_q$ starting at the current node.   
	In layer $l_{q+1}$ we have the output $y^{q+1}_{ic,j1}= \gad{\gad{x_{ic}=1} \rightarrow }$.
	The network output $y^r$ includes $\gad{y^{\hat{i}}_{ic}=0}$ and, thus, it holds that
	if $N_\mathcal{C}=0$ that all nodes $v$ of $G$ satisfy the properties of the $f$ gadgets if $v$ is of color $c \in C_i$.
	
\end{proof}
